# Supplementary material for: Stick-Slip Contact Line Motion on Kelvin-Voigt Model Substrates
Source: arXiv:2201.04189 ancillary file (2022-01-11)
Supplement: Supplementary file 1 [file StickSlipKV_supplement.pdf]

,

# Stick-Slip Contact Line Motion on Kelvin-Voigt Model Substrates

## Supplementary Material

Dominic Mokbel,[1] Sebastian Aland,[1,2] and Stefan Karpitschka[3]

[1] *HTW Dresden, Friedrich-List-Platz 1, 01069 Dresden, Germany*
[2] *TU Bergakademie Freiberg, Akademiestrasse 6, 09599 Freiberg, Germany*
[3] *Max Planck Intitute for Dyanmics and Self-Organization (MPIDS), 37077 Göttingen, Germany*

## I. FEM SIMULATIONS

The numerical simulation of soft wetting dynamics is a challenging problem since the representation of fluid/fluid and fluid/solid interface typically require fundamentally different numerical techniques. Additionally, the strong coupling of hydrodynamics and substrate dynamics near the contact line imposes stability restrictions and calls for special numerical schemes. First stable numerical methods for such problems appeared only very recently [1–3]. The first numerical method which can handle substrate viscoelasticity was presented in [2] and was used in this work. The key ingredients of the method are summarized in the following.

The computational domain $\Omega$ is seperated into a solid domain $\Omega_s$ for the substrate and a fluid domain $\Omega_f$ for both liquid and ambient. The fluid-solid interface $\Gamma$ is sharp. In contrast, the liquid-ambient interface is captured using an order parameter $\varphi$ referred to as phase field, which is defined in the fluid domain. The phase field differs between $\varphi = 1$ in the liquid and $\varphi = 0$ in the ambient. Across the liquid-ambient interface the phase field varies smoothly, following a tangent hyperbolic profile. Thus the interface has a finite thickness, which we can identify with the traction distribution $\epsilon$ mentioned in the previous sections.

Let us first summarize briefly the principal features of the model [2] including governing equations and numerical treatment. After that we consider the specifications needed for the application in this work.

### A. Governing equations

The system of Navier-Stokes and Cahn-Hilliard equations for the fluid domain reads

$$\left.\begin{aligned} \rho_f(\varphi)\left(\partial_t \mathbf{v}_f + \mathbf{v}_f \cdot \nabla \mathbf{v}_f\right) - \nabla \cdot \mathbf{S}_f &= \mathbf{F} \\ \nabla \cdot \mathbf{v}_f &= 0 \\ \partial_t \varphi + \mathbf{v}_f \cdot \nabla \varphi &= \nabla \cdot (m \nabla \mu) \\ \mu &= \tilde{\gamma}\epsilon^{-1} W'(\varphi) - \tilde{\gamma}\epsilon \Delta \varphi \end{aligned}\right\} \text{ in } \Omega_f \tag{1}$$

with viscous, pressure and capillary stress

$$\mathbf{S}_f = \eta_f(\varphi)\left(\nabla \mathbf{v}_f + \nabla \mathbf{v}_f^T\right) - p_f \mathbf{I} - \underbrace{\tilde{\gamma}\epsilon \nabla\varphi \otimes \nabla\varphi}_{\mathbf{S}_{\mathrm{ca}}} , \tag{2}$$

with (common) velocity field $\mathbf{v}_f$, phase-dependent density $\rho_f$ and viscosity $\eta_f$, and (scaled) liquid-ambient surface tension $\tilde{\gamma}$. The physically motivated surface tension $\gamma$ results from the relation $\tilde{\gamma} = 3\sqrt{2}\gamma$ where the scaling depends on the choice of the double well potential, which we set here $W(\varphi) = \varphi^2 (1-\varphi)^2$.

For the elastic solid, we take advantage of the fact that we actually consider gel-like materials. We suppose incompressibility and linear elasticity. The equations of momentum and mass conservation are

$$\left.\begin{aligned} \rho_s\left(\partial_t \mathbf{v}_s + \mathbf{v}_s \cdot \nabla \mathbf{v}_s\right) - \nabla \cdot \mathbf{S}_s &= \mathbf{F} \\ \nabla \cdot \mathbf{v}_s &= 0 \end{aligned}\right\} \text{ in } \Omega_s \tag{3}$$

with viscous, pressure and elastic stress

$$\mathbf{S}_s = \eta_s\left(\nabla \mathbf{v}_s + \nabla \mathbf{v}_s^T\right) - p\mathbf{I} + \underbrace{G_0\left(\nabla \mathbf{u} + \nabla \mathbf{u}^T - \nabla \mathbf{u}^T \nabla \mathbf{u}\right)}_{\mathbf{S}_{\mathrm{el}}} \tag{4}$$

with velocity $\mathbf{v}_s$, elastic shear modulus $G_0$ and a displacement field $\mathbf{u}$. The latter is the difference between current coordinates $\mathbf{x}$ and initial coordinates $\hat{\mathbf{x}}$ of material points, which we calculate by memorizing initial coordinates of each grid point and moving the solid grid with $\mathbf{v}_s$. Note that with this model we simulate a Kelvin-Voigt material, where $G_0$ and $\eta_s$ contribute in parallel to the solid stress.

Finally we consider the coupling conditions on the solid surface $\Gamma$.

$$\left.\begin{aligned} \mathbf{v}_f &= \mathbf{v}_s \\ \mathbf{S}_f \cdot \mathbf{n} &= \mathbf{S}_s \cdot \mathbf{n} + \nabla_\Gamma \cdot \left(\gamma_s\left(\varphi\right)\mathbf{P}\right) \\ 0 &= \tilde{\gamma}\epsilon\mathbf{n}\cdot\nabla\varphi + \gamma_s'\left(\varphi\right) \\ \mathbf{n}\cdot\nabla\mu &= 0 \end{aligned}\right\} \text{ on } \Gamma \ , \tag{5}$$

The first equation is a no slip-condition which gives us a common velocity field in whole $\Omega$. The second equation describes the balance of forces with the phase-dependent solid surface tension $\gamma_s\left(\varphi\right)$ which represents the tension along $\Gamma$ between the solid and the fluid. This is where solid-liquid tension $\gamma_1$ and solid-ambient tension $\gamma_0$ come into play. We use the following differentiable function of the phase field $\gamma_s\left(\varphi\right) = \left(\gamma_1 - \gamma_0\right)\varphi^2\left(3 - 2\varphi\right) + \gamma_0$, which implies $\gamma_s(0) = \gamma_0$ and $\gamma_s(1) = \gamma_1$. However, in this study $\gamma_0 = \gamma_1 = \gamma_s$. Furthermore, $\mathbf{n}$ denotes the outer normal to $\Omega_f$, $\nabla_\Gamma\cdot$ the surface divergence operator and $\mathbf{P} = \mathbf{I} - \mathbf{n}\otimes\mathbf{n}$ the surface projection operator. The third equation is a (static) contact angle condition. Note that this could be easily extended to a dynamic version, which we do not consider here. The last equation ensures mass conservation on $\Gamma$.

Let us emphasize here in particular that with this model approach we are able to avoid contact line singularities. The fact that the liquid-ambient interface is not represented by specific grid points brings the decisive advantage that the contact line can move freely along the substrate. The diffuse liquid-ambient interface is not pinned to the substrate surface $\Gamma$. The movement of the liquid-ambient interface is controlled by the Cahn-Hilliard diffusion which is constructed from energetic arguments, such as to realize the correct contact angles. This means that, for example, sliding of the liquid-ambient interface over the substrate is possible.

### B. Numerical treatment

The domains $\Omega_s$ and $\Omega_f$ are discretized on numerical grids which are matched at the interface $\Gamma$. This procedure enables a unified stable solution approach [2] in which all equations are assembled in a monolithic system. Momentum and mass balance equations are discretized by standard P2/P1 Taylor-Hood elements (polynomial basis functions of degree two and one for velocity and pressure, respectively). A special extended finite-element space is used to resolve the discontinuity of the pressure field across $\Gamma$. Cahn-Hilliard equations are discretized with P2 elements. To accommodate shape changes of the solid substrate the discretization is performed on a moving finite-element grid using the Arbitrary-Lagrangian-Eulerian (ALE) method. Movement of the substrate is imposed conforming with the velocity such that the substrate grid represents material points. Movement of the surrounding fluid grid follows surface motion by harmonically extending substrate deformations into the fluid phases. Further details about the numerical method can be found in [2].

### C. Test setup

The model just presented can be used for our test setup, which is illustrated in Fig. 1 (a) of the main manuscript. A cylinder hollow inside is shown, with radius $R = 2\,\mathrm{mm}$ in the hollow space and a casing with thickness $h_s = 1\,\mathrm{mm}$. The length of the cylinder is $6\,\mathrm{mm}$. This cylindrical structure allows for the use of rotational symmetry and thus the simulation of a 3D scenario in a 2D computational domain (see [2], Appendix). Consequently, the computational complexity significantly reduces compared to non-symmetrical 3D setups.

The cylinder casing itself is modelled as Kelvin-Voigt material. The hollow space is filled with fluid. Since we want to study the evolution of the contact line independently of a gradient in fluid viscosity, we assume a constant fluid viscosity $\eta_f = 1\,\mathrm{mPa\ s}$ in both liquid and ambient phase. Nevertheless we keep the terms "liquid" and "ambient" in the following. Furthermore we neglect inertia by setting the density $\rho_f = 0\,\mathrm{kg/m^3}$ everywhere, which reduces Eq. $(1)_1$ to the Stoke's equation. The remaining parameters are chosen as mentioned in Table 1 of the main manuscript.

As indicated in Fig. 1 (a) of the main manuscript we simulate the inflow of the liquid phase into the hollow space of the cylinder. Therefore we initially place the liquid-ambient interface $1\,\mathrm{mm}$ away from the inflow boundary $B_I$. At the inflow boundary we set a condition for velocity $\mathbf{v}_f = (v_Z,\ \ v_R)$ with the components $v_Z$ in flow direction and $V_R$

in lateral direction, respectively. Motivated by a parabolic flow profile, the condition reads

$$\mathbf{v}_f = \big(V(R^2 - x_R^2),\ \ 0\big)^T \qquad \text{on } B_I, \tag{6}$$

where $x_R$ is the position in lateral direction ($x_R = 0$ for $R = 0$) and $V$ is a factor which controls the (average) liquid-ambient interface velocity $\overline{v}$. The latter can be calculated in the rotational setup by

$$\overline{v} = \frac{\int_{\Omega_f} v_Z\, x_R}{\int_{\Omega_f} x_R}\ . \tag{7}$$

Furthermore we set $\mathbf{v}_s$=0 at the outer surface of the cylinder, $\delta\Omega_s\backslash\Gamma$, and $v_R = 0$ along the inflow and outflow, $\delta\Omega_f\backslash\Gamma$. Note, that $B_I \subset \delta\Omega_f$ and that the inset of Fig. 1 (a) of the main manuscript only shows a section of the rectangular computational domain in the vicinity of the contact line. In particular, the height of the actual domain $\Omega_f \cup \Omega_s$ is $R + h_s$ and the axis of symmetry is part of $\delta\Omega_f$.

Moreover, an important comparative quantity is the liquid-ambient interface rotation angle $\phi$ at the contact line, which can be defined in multiple ways. Here we measure $\phi$ as indicated in the inset of Fig. 1 (a) of the main manuscript. In the initial state this angle is zero as the liquid-ambient interface is vertical at the contact line. As the interface evolves, it curves accordingly. We performed automated angle measurement in a thin domain $A \subset \Omega_f$ in the direct vicinity of the contact line. The dimensions of $A$ are chosen to be negligibly small compared to the radius of curvature of the liquid-ambient interface. The angle $\phi$ is then calculated via a phase-dependent averaged normal

$$\mathbf{n}_a = \frac{\int_A \nabla\phi}{\int_A |\nabla\phi|}$$

which points towards the liquid phase. Consequently the angle is calculated by $\phi = \frac{\pi}{2} - \arccos\left(\mathbf{n}_a \cdot \mathbf{t}\ /\ |\mathbf{n}_a|\right)$, where $\mathbf{t}$ denotes the vertical. Note that we choose $\mathbf{t}$ in a way that $|\mathbf{t}| = 1$ and $\phi \geq 0$.

Fig. 1 (b) of the main manuscript compares the (sharp) stationary profiles of the solid substrate for different interface velocities with the analytical model, with excellent agreement. Note that we use the scaled profile height h/$(\gamma/G_0)$, the scaled position x/$h_s$ and the scaled velocity $\overline{v}/v_\ell$ which nondimensionalize the occuring physical quantities.

## II. ANALYTICAL CALCULATION

In the analytical calculation we assume translational symmetry along one surface direction, i.e. the 2D problem. We expect this geometry to be in close quantitative agreement with the FEM simulations since the deformations are much smaller than the cavity radius. We follow the Fourier-Transform approach of [4], and calculate substrate shapes according to [5] in the framework of linear viscoelasticity.

The Kelvin-Voigt material from the FEM simulations is described by a complex modulus

$$\widehat{\Psi}(\omega) = G_0 + i\,\omega\,\eta_s \tag{8}$$

where $G_0$ is the zero-frequency shear modulus and $\eta_s$ is the effective substrate viscosity.

Modelling the traction due to the moving liquid-liquid interface by a concentrated line load,

$$T(x,t) = \gamma\,\delta(x - v\,t), \tag{9}$$

leads to a dissipation singularity and a log-singular deformation profile [5]. In the phase-field representation, the liquid-liquid interface naturally has a width $\epsilon$, and one can derive the corresponding traction distribution for an equilibrium interface as

$$T(x) = \frac{3\gamma}{4\sqrt{2}\,\epsilon}\left(1 - \tanh^2\left(\frac{x - vt}{\sqrt{2}\,\epsilon}\right)\right)^2, \tag{10}$$

which indeed regularizes the dissipation singularity at a scale $\epsilon$. This allows one to calculate an effective substrate inclination under the contact line. The physically meaningful effective inclination is given by the weighted mean of the local slopes, using the normalized force distribution as weight.

We scale all horizontal lengths by the substrate thickness $h_s$ and, accordingly, the wave vector $q$ with $1/h_s$:

$$x = h_s\,x', \tag{11a}$$

$$q = \frac{q'}{h_s}. \tag{11b}$$

Time shall be scaled with $\tau = \eta_s/G_0$, the time scale of the KV solid and thus $\omega$ is scaled by $1/\tau$:

$$t = \tau\, t' \tag{12a}$$

$$\omega = \frac{\omega'}{\tau}. \tag{12b}$$

The solid profile height then scales as

$$h = \ell\, h', \tag{13}$$

with

$$\ell = \frac{\gamma}{G_0}, \tag{14}$$

the elastocapillary length. The remaining dimensionless geometry parameter is the elastocapillary number

$$\alpha_s = \frac{\gamma_s}{G_0\, h_s}, \tag{15}$$

which compares the solid elastocapillary length $\gamma_s/G_0$ to the thickness $h_s$ of the substrate.

In dimensionless units, the Green's function that relates the surface profile to the applied traction is (primes omitted from now on)

$$\widetilde{\mathcal{G}}(q) = \frac{1}{2\,q}\,\frac{2q - \sinh 2q}{1 + 2q^2 + \cosh 2q}, \tag{16}$$

which, in the limit $h_s \to \infty$, recovers the Green's function for the infinitely thick elastic layer. The complex modulus becomes, in scaled quantities,

$$\widehat{\psi}(\omega) = 1 + i\,\omega, \tag{17}$$

and the scaled traction in Fourier space is

$$\widehat{\widetilde{\mathcal{T}}}(q,\omega) = \frac{\pi^2}{\sqrt{2}}\, q\epsilon\left(q^2\epsilon^2 + 2\right)\operatorname{csch}\left(\frac{\pi q \epsilon}{\sqrt{2}}\right)\,\delta(\omega + v\,q), \tag{18}$$

where $\epsilon$ is scaled by $h_s$, like all horizontal dimensions. The solution for the surface profile in the co-moving frame reads:

$$\widehat{\widetilde{h}}(q,v) = \frac{\widehat{\widetilde{\mathcal{T}}}(q,-v\,q)}{\widehat{\psi}(-v\,q)/\widetilde{\mathcal{G}}(q) + \alpha_s\, q^2}. \tag{19}$$

The inverse Fourier transform to real space is performed numerically. Table 1 of the main manuscript lists the parameters used in the numerical inversion.

Figure 1 shows the substrate slope at the contact line for various interface widths $\epsilon/\ell$. For small $\epsilon/\ell \ll 1$, the speed of maximum rotation converges to a value on the order of the elastocapillary velocity $v_\ell$. For intermediate $\epsilon/\ell < 1$, a slight variation of the location of the maximum is observed. In the simulations, $\epsilon$ is kept constant and $\ell$ is varied. Thus the onset of stic-slip motion is expected to depend slightly on $\ell$.

### A. Comparison of simulation results to the analytical model

We validate the substrate deformations obtained in the numerical simulation by a direct comparison to the analytical model. Figure 2 (left) shows the characteristic, velocity-dependent dimensions of the wetting ridge. On the right panel, we compare the simulated maximum ridge height, $h_{max}$, to the analytical model, finding an excellent agreement, both for small and large speeds where the contact line moves at constant speed. In the stick-slip regime, the ridge shapes change drastically over one cycle, ruling out a direct comparison between the models.

Due to the strong dissipation in a Kelvin-Voigt solid, which is regularized by the finite width of the capillary traction, the maximum ridge height is not located at the contact line, but behind it. The distance between the contact line and the peak of the ridge, in vertical and in horizontal directions, are plotted in Fig. 3. $\Delta h$ shows a pronounced maximum at the elastocapillary velocity. $\Delta x$ increases monotonically and saturates at large speeds. Also for these ridge properties, we find an excellent agreement between the two models.

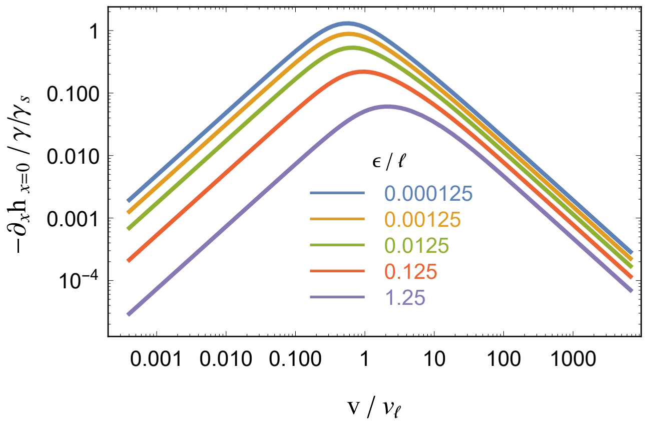


FIG. 1: Substrate slope at the contact line, calculated with the analytical model, for different $\epsilon/\ell$.

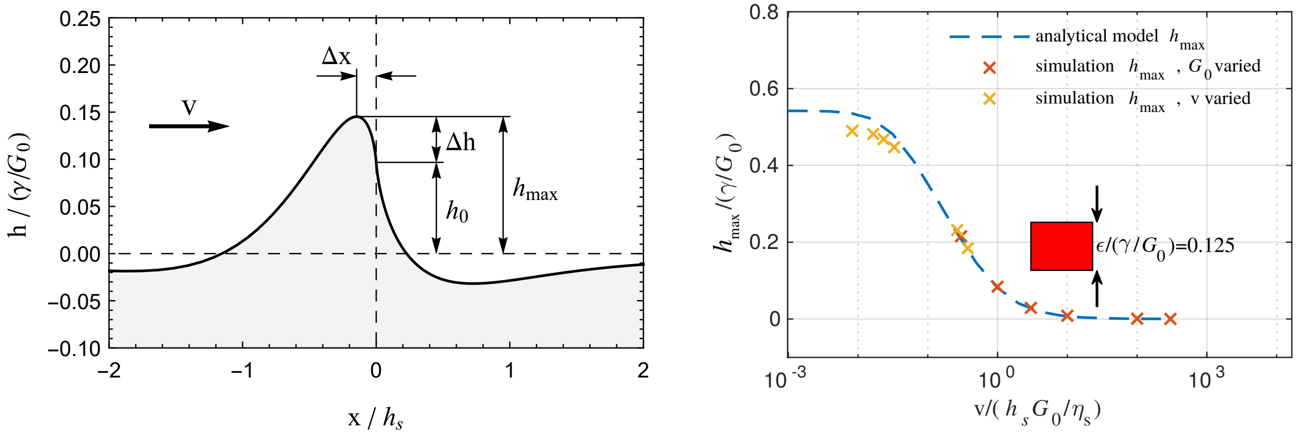


FIG. 2: Left: Characteristic dimensions of a moving wetting ridge. The highest point of the ridge is not located at the contact line, but $\Delta x$ behind and $\Delta h$ above the contact line, due to strong dissipation in the solid. Both $h_0$ and $h_{max}$ decrease with speed, due to dissipation. Right: $h_{max}$ as a function of the imposed velocity, comparison between the analytical model (dashed line) and the simulations (markers). The gap at intermediate velocities is the stick slip region, where a comparison between the unsteady simulation results and the analytical model becomes impossible.

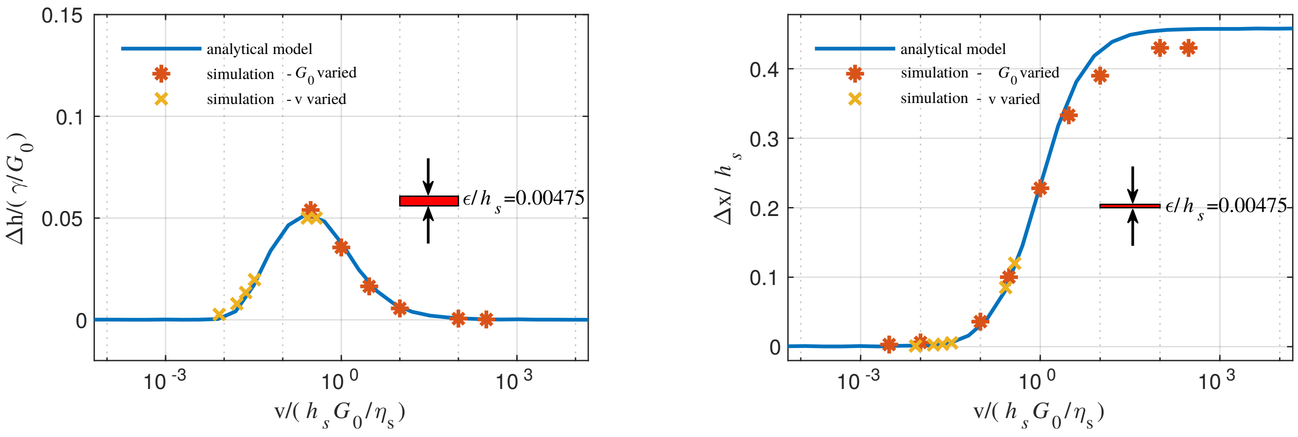


FIG. 3: $\Delta h$ (left) and $\Delta x$ as a function of imposed speed, comparing the analytical model to simulation results.

[1] E. Van Brummelen, T. Demont, and G. van Zwieten, International Journal for Numerical Methods in Engineering **122**, 5331 (2021).
[2] S. Aland and D. Mokbel, International Journal for Numerical Methods in Engineering **122**, 903 (2021).
[3] S. Aland and P. Auerbach, International Journal for Numerical Methods in Engineering (2021).
[4] D. Long, A. Ajdari, and L. Leibler, Langmuir **12**, 5221 (1996).
[5] S. Karpitschka, S. Das, M. van Gorcum, H. Perrin, B. Andreotti, and J. Snoeijer, Nat. Commun. **6**, 7891 (2015).
